# Supplementary material for: BootSeer: Analyzing and Mitigating Initialization Bottlenecks in Large-Scale LLM Training
Source: arXiv:2507.12619 source file (2026-01-27)
Supplement: Supplementary file 1 [file appendix.tex]

\section{Hello World}
%\subsection{Hello World}
